# Supplementary material for: Generating Content for HDR Deghosting from Frequency View
Source: arXiv:2404.00849 source file (2024-04-01)
Supplement: Supplementary file 1 [file X_suppl.tex]

\clearpage
\setcounter{page}{1}
\maketitlesupplementary

\section{Model Details}
\begin{figure}[tb]
\centering
% \footnotesize \quad\qquad\qquad\qquad AHDR \cite{yan2019attention} \qquad ~DDPM \cite{pmlr-v37-sohl-dickstein15} \qquad\quad Our 
\includegraphics[width=1\linewidth]{suppl/ahdr.png}
\caption{We using the attention module from AHDR \cite{yan2019attention} as the alignment module. Here, $X_i$ represents 6-channel LDR images, and the output features have $C=60$ channels.}
\label{ahdr}
\vspace{-0.4cm}
\end{figure}
\noindent \textbf{Denoising Network:} 
The network architecture is a modified version of the U-Net found in DDPM \cite{NEURIPS2020_4c5bcfec}; As shown in Fig.~\ref{dnframe}, we replace the original DDPM residual blocks with slightly modified nonlinear activation free blocks (NAFBlocks)\cite{luo2023refusion}.
Nonlinear activation free means that we replace all nonlinear activation functions with the “SimpleGate”, an element-wise operation that splits feature channels into two parts and then multiplies them together to produce the output. As illustrated in Fig.\ref{dnframe}, to make the model share parameters across time, we add an additional multilayer perceptron to process the time embedding to channel-wise scale and shift parameters $\gamma$ and $\beta$, for both the attention layer and feed-forward layer.
% To make the model share parameters across time, we transform the timestep through sinusoidal positional encoding and fuse these embeddings to each residual block through an MLP. 
In practical applications, we select $C=32$, and employ four resolution depths in the U-Net architecture, with channel multipliers of $\{1,2,4,8\}$. In both the encoder and decoder, each stage comprises two NAFBlocks, while the middle stage specifically consists of one NAFBlock.
This results in the entire denoising network containing $1.76M$ parameters. 

\noindent \textbf{DHRNet:} 
DHRNet is comprised of multiple stacked Reconstruction Blocks, each including one Prior Integration Module (PIM) \ref{dhrframe} (a) and several Feature Refinement Modules (FRM) \ref{dhrframe} (b). In practical applications, the number of FRMs in each block is set to 3, and C is configured as 60. In PIM, N is set to 3. The downsampling kernel sizes for avgpool in PIM and FRM are set as 4 and 2, respectively. It is noteworthy that DHRNet does not directly utilize LDR images as input; instead, it employs an alignment module (AM) to obtain implicitly aligned features as input. As depicted in Fig.~\ref{ahdr}, we utilize the Attention Network from AHDR \cite{yan2019attention} to process various LDR images, extracting implicitly-aligned features for input to DHRNet. 

\section{Algorithm}
\begin{algorithm*}[h]
\caption{DM Training}

\label{alg:A}  
\begin{algorithmic}[1]
\REQUIRE~~\\  LDRs-HDR image pairs $(X_i,H)$, \\Total diffusion step $T$, 
implicit sampling step $S$, Noise schedule $\beta_t(t \in[1, T])$.
\STATE \textbf{Initialize:} $\alpha_t=1-\beta_t, \bar{\alpha}_T=\prod_{i=0}^T \alpha_i$
\STATE \textbf{Initialize:} The DHRNet (contains AM and Conv$3\times3$ behind DHRNet) of LF-Diff copies the parameters of trained LF-Diff from stage one.
\REPEAT
\STATE $t \sim Uniform\{1,\cdots,T\}$
\STATE $\epsilon_t\sim \mathcal{N}(0,\mathbf{I})$
\STATE $\left.z=\text { LPENet (PixelUnshuffle }\left(\text { Concat }\left(H, \mathcal{T}\left(H\right)\right)\right)\right)$ 
\STATE $\mathbf{D}=\operatorname{LPENet}_{D M}\left(A M\left(\text { PixelUnshuffle }\left(X_i\right)\right)\right)$ 
\STATE $z_0=z$ 
\STATE Take gradient descent step on $\mathbb{E}_{t,z_0,\epsilon_t}[\Vert\epsilon_t-\epsilon_{\theta}(\sqrt{{\bar{\alpha}_t}}z_0+\sqrt{1-\bar{\alpha}_t}\epsilon_t,t,D)\Vert^2]$ 
\STATE $\hat{\mathbf{z}}_T \sim \mathcal{N}(\mathbf{0}, \mathbf{I})$
\FOR{$i = S:1$}  
\STATE $t=(i-1) \cdot T / S+1$
\STATE $t_{\mathrm{next}}=(i-2) \cdot T / S+1$ if $i>1$, else 0
\STATE $  \hat{\mathbf{z}}_{t_{next}} \leftarrow \sqrt{\bar{\alpha}_{t_{\text {next }}}}\left(\frac{\hat{\mathbf{z}}_t-\sqrt{1-\bar{\alpha}_t} \cdot \epsilon_\theta\left(\hat{\mathbf{z}}_t, D, t\right)}{\sqrt{\bar{\alpha}_t}}\right)+  \quad \sqrt{1-\bar{\alpha}_{t_{\text {next }}}} \cdot \epsilon_\theta\left(\hat{\mathbf{z}}_t, D, t\right)$
\ENDFOR
\STATE $\hat{z}=\hat{z_0}$
\STATE Take gradient descent step on $\|\hat{z}-z\|_1$ 
\STATE $\hat{H}=Conv3\times 3 (DHRNet(AM(X_i),\hat{z}))$
\STATE Take gradient descent step on $\mathcal{L}_{r}$ (paper Eq. (11))

\UNTIL converged
\end{algorithmic}  
\end{algorithm*}

\begin{algorithm*}[h]
\caption{LF-Diff Inference}

\label{alg:B}  
\begin{algorithmic}[1]
\REQUIRE~~\\  LDRs images $X_i$, Total diffusion step $T$,
implicit sampling step $S$, \\Noise schedule $\beta_t(t \in[1, T])$, Trained LF-Diff
\STATE \textbf{Initialize:} $\alpha_t=1-\beta_t, \bar{\alpha}_T=\prod_{i=0}^T \alpha_i$
\STATE Reverse Process:
\STATE Sample $\hat{\mathbf{z}}_T \sim \mathcal{N}(\mathbf{0}, \mathbf{I})$
\STATE $\mathbf{D}=\operatorname{LPENet}_{D M}\left(A M\left(\text { PixelUnshuffle }\left(X_i\right)\right)\right)$
\FOR{$i = S:1$}
\STATE $t=(i-1) \cdot T / S+1$
\STATE $t_{\mathrm{next}}=(i-2) \cdot T / S+1$ if $i>1$, else 0
\STATE $  \hat{\mathbf{z}}_{t_{next}} \leftarrow \sqrt{\bar{\alpha}_{t_{\text {next }}}}\left(\frac{\hat{\mathbf{z}}_t-\sqrt{1-\bar{\alpha}_t} \cdot \epsilon_\theta\left(\hat{\mathbf{z}}_t, D, t\right)}{\sqrt{\bar{\alpha}_t}}\right)+  \quad \sqrt{1-\bar{\alpha}_{t_{\text {next }}}} \cdot \epsilon_\theta\left(\hat{\mathbf{z}}_t, D, t\right)$
\ENDFOR
\STATE $\hat{z}=\hat{z_0}$
\STATE $\hat{H}=Conv3\times 3 (DHRNet(AM(X_i),\hat{z}))$
\STATE Output reconstructed HDR image $\hat{H}$
\end{algorithmic}  
\end{algorithm*}
Our LF-Diff consists of two training stages. After completing the first pretraining phase for LF-Diff, the algorithm for the second stage LF-Diff training is outlined in Algorithm \ref{alg:A}. The algorithm for LF-Diff inference is summarized in Algorithm \ref{alg:B}.

\section{Perceptual Metrics}
As indicated in Table \ref{pm}, we additionally computed various common perceptual metrics, including FID \cite{heusel2017gans}, LPIPS \cite{zhang2018unreasonable}, VSI \cite{zhang2014vsi}, and AHIQ \cite{lao2022attentions}. Due to the domain differences between HDR images and natural images, tonemapping was applied to both the generated results and ground truth (GT) for computing perceptual metrics. This approach enables a more accurate evaluation of the quality of the generated images. It can be observed that, compared to DNN-based methods, DDPM-based methods typically exhibit superior perceptual metrics. Our approach maintains excellent perceptual metric performance while being 10$\times$ faster than the previous diffusion-model-based method DiffHDR.

\section{Additional Qualitative Results}
In this section, we present additional qualitative results that we did not show in the main text due to the limited space of paper. In Figs. \ref{compare1} show visual results for various motion cases in Kalantari's dataset \cite{Kalantari2017Deep} and Hu's dataset \cite{hu2020sensor}. Fig. \ref{compare2} and \ref{compare3} provide additional qualitative results without ground truth.

\begin{figure*}[t]
\centering
\includegraphics[width=\textwidth]{suppl/supp_dn.png}
\caption{The diagram illustrates the U-Net architecture used for the Denoising Network. The dimensions W, H, and C correspond to the width, height, and number of channels of the features respectively. }
\label{dnframe}
\end{figure*}

\begin{figure*}[htbp]
\centering
\includegraphics[width=\textwidth]{suppl/DHRNet.png}
\caption{DHRNet consists of two modules: a Prior Integration Module (PIM) that fuses the LPR with intermediate features of DHRNet, and a Feature Refinement Module (FRM) that further processes the fused features to HDR image.}
\label{dhrframe}
\end{figure*}

\begin{table*}[t]
\caption{Quantitative comparison of proposed network with several state-of-the-art methods on Kalantari's \cite{Kalantari2017Deep} datasets.}
\begin{tabular}{c|ccccccccc}
\toprule
Models & GT  & Hu\cite{Hu2013deghosting} & Kalantari\cite{Kalantari2017Deep} & AHDR\cite{yan2019attention}   & HDRGAN\cite{niu2021hdr} & ADNet\cite{liu2021adnet}  & CA-ViT\cite{liu2022ghost} & DiffHDR\cite{10288540} & Ours   \\ \midrule
FID $\downarrow$    & 0   & 37.27  & 33.3      & 9.43   & 9.32   & 12.42  & \underline{5.91}   & 6.20     & \textbf{5.73}   \\
LPIPS $\downarrow$  & 0   & 0.0302 & 0.0341    & 0.0166 & 0.0159 & 0.0169 & 0.0132 & \underline{0.0109}  & \textbf{0.0099} \\
VSI $\uparrow$    & 100 & 96.38  & 98.27     & 99.13  & 99.3   & 98.97  & 99.36  & \underline{99.48}   & \textbf{99.52}  \\
AHIQ $\uparrow$   & 50  & 34.07  & 42.61     & 46.83  & 47.2   & 46.6   & 46.57  & \underline{47.82}   & \textbf{47.84}  \\ \bottomrule
\end{tabular}
\label{pm}
\end{table*}

\begin{figure*}[h]
\centering
\includegraphics[width=\textwidth]{suppl/wgt0.jpg}
\caption{Qualitative results for various motion cases on the Kalantari's dataset \cite{Kalantari2017Deep} and Hu's dataset \cite{hu2020sensor}.}
\label{compare1}
\end{figure*}

\begin{figure*}[h]
\centering
\includegraphics[width=\textwidth]{suppl/wgt3.png}
\caption{Qualitative results for various motion cases on the Tursun \etal \cite{tursun2016objective} dataset.}
\label{compare2}
\end{figure*}

\begin{figure*}[h]
\centering
\includegraphics[width=\textwidth]{suppl/wgt2.png}
\caption{Qualitative results for various motion cases on the Tursun \etal \cite{tursun2016objective} dataset.}
\label{compare3}
\end{figure*}
